# Supplementary material for: Exploring the Potential of ChatGPT in Automated Code Refinement: An Empirical Study
Source: arXiv:2309.08221 source file (2023-09-15)
Supplement: Supplementary file 1 [file sec08-appendix.tex]

\section{Appendix}

%remove all content here to website
This is the appendix section.

\subsection{Prompts Settings}

All 5 prompts.

\subsection{ChatGPT RootCause and Fix Examples}
Different Types of Root Causes, and 3 fix methods for them.

\subsection{ChatGPT Maybe right Examples}
Cases that ChatGPT gives answers that different from ground truth answers, but may be right after evaluation. Alternative solutions or even better solutions.

This is the second subsection in the appendix.
